# Supplementary material for: Safety, Trust, and Ethics Considerations for Human-AI Teaming in Aerospace Control
Source: arXiv:2311.08943 source file (2023-11-15)
Supplement: Supplementary file 1 [file Appendix.tex]

The unsafe control actions, scenarios, and requirements in this section represent the current work in progress over a multi-year effort. As such, requirements in particular are at an early research stage, and alternative requirements may also meed the needs of preventing unsafe control actions. 

\subsection{L2W1: Level 2 Wingman Signal 1: Neural Network to Run Time Assurance}
The NNCS receives lead and wingman state information from the airframe and computes a set of control commands that are sent to the RTA block.

\begin{table}[hbt!]
\begin{center}
\caption{\label{t:STPA_W1} W1: Neural Network Control System to Run Time Assurance}
\begin{tabular}[t]{|L{4.5cm} | L{5cm} | L{5.5cm} |}
\hline
\textbf{Unsafe Control Action}	&	\textbf{Rationale / Scenario}	&	\textbf{Requirement}	\\\hline
NNCS \textbf{provides} a command to the RTA that would a loss of safe separation [H1], loss of control [H2], violation of geofence [H3], or harm to the pilot or aircraft [H4], or violate EPM limits, terminating testing early [H6].   
    & This could occur due to training that does not consider safety constraints.
	& [RL2.W1.1] The NNCS shall be trained with penalties that account for soft safety constraints and EPM limits, and/or an RTA should be used during the training process.  \\\hline
NNCS \textbf{does not provide} a control command to the RTA.   
    & This could occur due to a fault in the NNCS component.
	& [RL2.W1.2] In the presence of an NNCS fault, a default value shall be output from the NNCS.  \\\hline
	& & [RL2.W1.3] The pilot shall be notified of NNCS faults (via W13).\\\hline 
NNCS \textbf{does not provide} data to be recorded to the on-board database [H5].
    & Failing to record NNCS data could happen due to a design flaw or running out of time within the timeframe to send the data. 
	& [RL2.W1.4]The data recorded about NNCS activation shall be identified and checked. It should also be determined whether the NNCS has sufficient time within a specific operation frame on operational hardware to complete it's function as well as send data to be recorded. If the data cannot be recorded, the pilot or test engineer shall be alerted.  \\\hline
NNCS \textbf{is too early or too late to provide} a control command to the RTA, resulting in test failure [H6] or flight instability [H2].   
    & NNCS could send an early or late signal if the NNCS falls out of sync with the airframe and RTA.  
	& [RL2.W1.5] The NNCS, Airframe, and RTA shall be synchronized (e.g. reference the same clock)\\\hline
\end{tabular}
\end{center}
\end{table}

\newpage
\subsection{L2W2: Level 2 Wingman Signal 2: Run Time Assurance to Control Selector}
%The RTA receives an observation of the current aircraft state from the airframe, on/off and settings from the operator, and control commands from the NNCS. The RTA sends a filtered pitch, roll, speed, and yaw control commands that ensure collision avoidance (safe separation) and geofence satisfaction to the CS; status to the pilot/engineer. %
%
The RTA is responsible for assuring collision freedom and geofence adherence within the limits if the EPM. %The RTA does not monitor soft safety constraints. The proposed RTA design will begin by focusing on combining geofence and RTA as an initial proof of concept; however, future RTA designs should consider inclusion of jetwash avoidance. As the design currently stands, the responsibility of jetwash avoidance is placed on the human safety pilot. The EPM/Switch might also have a requirement to check reasonableness of input from RTA in the event that there is corruption between the RTA output and input to the EPM/Switch.

\begin{table}[hbt!]
\begin{center}
\caption{\label{t:STPA_W2_provides1} W2: Unsafe control actions between the RTA and Control Selector: Provides (1 of 2)}
\begin{tabular}[t]{|L{4.5cm} | L{5cm} | L{5.5cm} |}
\hline
\textbf{Unsafe Control Action}	&	\textbf{Rationale / Scenario}	&	\textbf{Requirement}	\\\hline
RTA \textbf{provides} a control command to control selector when the command violates safe separation [H1], causes loss of control [H2], violates geofence [H3], causes harm to the pilot or aircraft [H4].
    & Sending an unsafe command could occur because the aircraft is outside of expected operational conditions. For example, the angle of attack of the aircraft could be outside the RTA design range the RTA.
	& [RL2.W2.1] The RTA shall be designed to provide geofence and collision avoidance within the entire range of EPM limits.	\\\hline
     & Sending an unsafe command could occur due to a fault in the lead position report, wingman position report, or entity reports (a fault in W4). 
	& [RL2.W2.2] The RTA shall check the reasonableness of inputs based on history and aircraft limits. If an unreasonable input is found, the RTA shall alert the safety pilot that the RTA is in a failed state via W7.  \\\hline
	& Sending an unsafe command could occur because no signal comes from the NNCS due to a fault (a fault in W1). 
	& [RL2.W2.3] In the absence of a signal from the NNCS, the RTA should use the last control command from the NNCS in the computation of an RTA response.   \\\hline
	& Sending an unsafe command could occur because no signal was ever output from the NNCS.  
	& [RL2.W2.4] When no last control command from the NNCS is available, RTA shall assume a maintain maneuver command based on the current state of the aircraft.   \\\hline
    & Sending an unsafe command could occur due to a fault the specification of the safe separation distance or geofence.
	& [RL2.W2.5] The units and data format for safe separation distance and geofence shall be reasonably obvious to the operator. Safe separation and geofence values input by the operator shall be checked for a reasonableness.\\\hline
\end{tabular}
\end{center}
\end{table}

\begin{table}[hbt!]
\begin{center}
\caption{\label{t:STPA_W2_provides2} W2: Unsafe control actions between the RTA and Control Selector: Provides (2 of 2)}
\begin{tabular}[t]{|L{4.5cm} | L{5.5cm} | L{5cm} |}
\hline
\textbf{Unsafe Control Action}	&	\textbf{Rationale / Scenario}	&	\textbf{Requirement}	\\\hline
RTA \textbf{provides} a control command to control selector when the command violates safe separation [H1], causes loss of control [H2], violates geofence [H3], causes harm to the pilot or aircraft [H4].
	& Sending an unsafe command could occur due to a fault in the RTA computation. 
	& [RL2.W2.6] The RTA computation shall be dual redundant \textit{and / or} checked for reasonableness properties \textit{and / or} the human safety pilot shall be prepared to take control during the test.\\\hline
	& Sending an unsafe command could occur due to a fault in transmission to the CS.
	& [RL2.W2.7] The output of the RTA shall be shall be dual redundant \textit{and / or} checked for reasonableness properties. 	\\\hline
	& Sending an unsafe command could occur due to a CS/RTA mismatch in units or data format. For example, a speed command given in ft/s when knots is expected. 
	& [RL2.W2.8] The output of the RTA shall adhere to the expected units and format of the CS.  		\\\hline
	& If the output trajectory puts the aircraft in the jetwash of the lead aircraft for some minimum amount of time, it could case the aircraft to lose control. 
	& [RL2.W2.9] Knowledge of jetwash is outside the scope of the RTA, and trajectories towards the jetwash of the lead aircraft should be monitored for safety by the safety pilot.	\\\hline
RTA \textbf{provides} a control command to control selector when the command violates the envelope monitored by the EPM, resulting in a loss of planned test [H6], or potential harm to the human pilot or aircraft [H4].
    & Sending an command outside the EPM unsafe command could occur because the aircraft is outside of expected operational conditions. For example, the angle of attack of the aircraft could be outside the range the RTA is designed for.
	& [RL2.W2.10] The RTA shall be designed to provide geofence and collision avoidance within the EPM limits.	\\\hline
\end{tabular}
\end{center}
\end{table}

\begin{table}[hbt!]
\begin{center}
\caption{\label{t:STPA_W2_too_late} W2: Unsafe control actions between the RTA and Control Selector: Timing (too late)}
\begin{tabular}[t]{|L{4.5cm} | L{5.5cm} | L{5cm} |}
\hline
\textbf{Unsafe Control Action}	&	\textbf{Rationale / Scenario}	&	\textbf{Requirement}	\\\hline
RTA \textbf{provides a late} a control command to control selector when necessary to provide safe separation [H1] or stay in geofence [H3].
    & RTA could send a late signal if the RTA and CS fall out of sync.  
	& [RL2.W2.11] The RTA and CS shall be synchronized (e.g. reference the same clock)\\\hline
RTA \textbf{provides a late} a control command to control selector when necessary to provide safe separation [H1] or stay in geofence [H3].
    & RTA could send a late signal if the computation time of the solution causes a frame overrun.
	& [RL2.W2.12] The RTA shall be able to compute a solution within a portion of the allotted frame rate.\\\hline
\end{tabular}
\end{center}
\end{table}

\newpage
\begin{table}[hbt!]
\begin{center}
\caption{\label{t:STPA_W2_does_not_provide} W2 Unsafe control actions between the RTA and Control Selector: Does Not Provide}
\begin{tabular}[t]{|L{4.5cm} | L{5.5cm} | L{5cm} |}
\hline
\textbf{Unsafe Control Action}	&	\textbf{Rationale / Scenario}	&	\textbf{Requirement}	\\\hline
RTA \textbf{does not provide} a control command to control selector when necessary to provide safe separation [H1] or stay in geofence [H3].
    & Failing to send control commands to assure collision protection and geofence could happen because of a data dropout between the RTA and the CS. 
	&  [RL2.W2.13] The CS shall alert the pilot (via W14) when no signal is received (from W2).\\\hline
    & Failing to send control commands to assure collision protection and geofence could happen because it is not possible to send a safe signal. 
	& [RL2.W2.14] The RTA should alert the pilot of a failure of the RTA is a safe command cannot be found.\\\hline
	& This could occur if the pilot or test engineer turns off the RTA and then turns it back on again mid-flight when it is already violating safe separation or geofence. 
	&  [RL2.W2.15] The interface to the pilot/test engineer will check if the geofence or safe separation is being violated when RTA is off, and will alert the pilot/test engineer before they turn the RTA back on. \\\hline
RTA \textbf{does not provide} data to be recorded to the on-board database [H5].
    & Failing to record RTA data could happen due to a design flaw or running out of time within the timeframe to send the data. 
	& [RL2.W2.16] The data recorded about RTA activation shall be identified and checked. It should also be determined whether the RTA has sufficient time within a specific operation frame on operational hardware to complete it's function as well as send data to be recorded. If the data cannot be recorded, the pilot or test engineer shall be alerted.  \\\hline
\end{tabular}
\end{center}
\end{table}

\newpage
\subsection{L2W3: Level 2 Wingman Signal 3: Control Switch to Airframe}
The control switch selects whether to send the NNCS/RTA or safety pilot signal to the airframe.

\begin{table}[hbt!]
\begin{center}
\caption{\label{t:STPA_W3} W3: Unsafe control actions between the CS and Airframe}
\begin{tabular}[t]{|L{4.5cm} | L{5cm} | L{5.5cm} |}
\hline
\textbf{Unsafe Control Action}	&	\textbf{Rationale / Scenario}	&	\textbf{Requirement}	\\\hline
CS \textbf{provides} a control command to the airframe when the command causes loss of control [H2] or causes harm to the pilot or aircraft [H4].
	& Sending an unsafe command could occur due to a fault in the CS switching. 
	& [RL2.W3.1] The CS should default to safety pilot control in the event of a fault.\\\hline
	& Sending an unsafe command could occur due to a fault in transmission to the airframe.
	& [RL2.W3.2] The output of the CS shall be shall be at least dual redundant \textit{and / or} checked for reasonableness properties. 	\\\hline
	& Sending an unsafe command could occur due to a CS/airframe mismatch in units or data format. For example, a speed command given in ft/s when knots is expected. 
	& [RL2.W3.3] The output of the CS shall adhere to the expected units and format of the airframe.  		\\\hline
	& Sending an unsafe command could occur because the aircraft is outside of expected operational conditions. For example, the angle of attack or roll angle could be outside the safe set for flight test.
	& [RL2.W3.4] The safety pilot shall provide control signals the keep the aircraft within safe operating conditions.	\\\hline
	& Sending an unsafe command could occur because an unsafe command came from the RTA due to a fault (a fault in W2). 
	& [RL2.W3.5] The EPM and Safety pilot shall provide sufficient redundant safety monitoring to switch when needed to mitigate RTA signal risks.   \\\hline
	& Sending an unsafe command could occur because no signal was ever output from the RTA.  
	& [RL2.W3.6] In the absence of a signal from the RTA, the CS shall default switch to safety pilot control.    \\\hline
CS \textbf{provides a late} a control command to airframe, resulting in a loss of control [H4].
    & CS could send a late signal if the CS and airframe fall out of sync.  
	& [RL2.W3.7] The CS and airframe shall be synchronized (e.g. reference the same clock)\\\hline
CS \textbf{does not provide} a control command to airframe resulting in a loss of control.
    & Failing to send control commands could happen because of a data dropout between the CS and the airframe. 
	& [RL2.W3.8] The signal from CS to the airframe shall be as reliable as practical through means such as redundancy.\\\hline
CS \textbf{does not provide} data to be recorded to the on-board database [H5].
    & Failing to record CS data could happen due to a design flaw or running out of time within the timeframe to send the data. 
	& [RL2.W3.9] The data recorded about CS state activation shall be identified and checked. It should also be determined whether the CS has sufficient time within a specific operation frame on operational hardware to complete it's function as well as send data to be recorded. If the data cannot be recorded, the pilot or test engineer shall be alerted.  \\\hline
\end{tabular}
\end{center}
\end{table}

\newpage
\subsection{L2W4: Level 2 Wingman Signal 4: Airframe State Output}
The Airframe outputs an updated state observation to the NNCS, RTA, EPM, Safety Pilot, and Test Engineer. Note that a redundant, heterogeneous source of truth is available to the the Safety Pilot and Test Engineer, because it is assumed that they have insight, beyond what is displayed in state information sensed by the airframe, i.e. the pilots can use what they see out the window as a sanity check to instrument readings.

\begin{table}[hbt!]
\begin{center}
\caption{\label{t:STPA_W4} W4: Airframe output}
\begin{tabular}[t]{|L{4.5cm} | L{5cm} | L{5.5cm} |}
\hline
\textbf{Unsafe Control Action}	&	\textbf{Rationale / Scenario}	&	\textbf{Requirement}	\\\hline
Airframe \textbf{provides} an incorrect estimation of state, which when acted on by the NNCS/RTA resulting in a control command that violates safe separation [H1], causes loss of control [H2], violates geofence [H3], causes harm to the pilot or aircraft [H4].
    & This could happen due to an error in an airframe sensor. 
	& [RL2.W4.1] The safety pilot shall check instrument readings and use visual situation assessment to provide redundant collision avoidance, geofence, and other safety monitoring.\\\hline
Airframe \textbf{does not provide} a state estimate through W4.
	& This could happen due to a fault or frame overrun in the estimation software, or a faulty sensor.
	& [RL2.W4.2] The NNCS and RTA shall be designed to experience a reasonable amount of noise or dropouts in the sensed state, also see previous requirement.\\\hline
Airframe \textbf{too late to provide} a state estimation through W4.   
    & The Airframe could send a signal too late if it falls out of with the NNCS, RTA, EPM or CS.  
	& [RL2.W4.3] The NNCS, Airframe, RTA, CS, and EPM shall be synchronized (e.g. reference the same clock)\\\hline
\end{tabular}
\end{center}
\end{table}

\newpage
\subsection{L2W5: Level 2 Wingman Signal 5: Pilot to CS}
The pilot is expected to constantly provide a backup signal to the CS parallel to the NNCS/RTA path, as well as to control the aircraft between test points.

\begin{table}[hbt!]
\begin{center}
\caption{\label{t:STPA_W5} W5: Pilot to Control Selector}
\begin{tabular}[t]{|L{4.5cm} | L{5cm} | L{5.5cm} |}
\hline
\textbf{Unsafe Control Action}	&	\textbf{Rationale / Scenario}	&	\textbf{Requirement}	\\\hline
Pilot \textbf{provides} a control command to CS that violates safe separation [H1], causes loss of control [H2], violates geofence [H3], causes harm to the pilot or aircraft [H4].
    & Sending an unsafe command could occur because the pilot is incapacitated or ability to react is impaired during the test (for example, the primary controller technically stays within safe boundaries but still imparts physiological stress). 
	& [RL2.W5.1] The safety pilot shall evaluate their health status prior to flight and terminate the NNCS/RTA control early if they suspect reasonable chance of impairment.\\\hline
	Pilot \textbf{provides} a control command to CS that violates safe separation [H1].
	& Sending an unsafe command could occur because the pilot has lost situational awareness (line of sight) to the lead.
	& [RL2.W5.2] The safety pilot shall maintain line of sight or intervene when line of sight is lost long enough for a potential collision [SSC1, SSC2].\\\hline
Pilot \textbf{does not provide} a control command to CS when needed to prevent loss of safe separation [H1], loss of control [H2], violation of geofence [H3], or harm to the pilot or aircraft [H4].
    &  This could occur due to a system fault that prevents transmission of the pilot command to the CS. 
	&  [RL2.W5.3] The signal from the pilot to the CS shall be as reliable as possible, likely having two to four redundant paths.\\\hline
Pilot \textbf{is too late to provide} a control command to prevent loss of safe separation [H1], loss of control [H2], violation of geofence [H3], or harm to the pilot or aircraft [H4].
    &  This could happen if the pilot safety pilot loses situation awareness due to distraction or loss of line of sight [SSC1,SSC2].
	&  [RL2.W5.4] The pilot should terminate the test if they become distracted or lose line of sight for too long.\\\hline
Pilot \textbf{is too early to provide} a control command to CS, when the NNCS/RTA is safe causing premature test termination and a loss of planned operations [H6].
    &  This could occur if the pilot is not well versed in the RTA and EPM safety limits prior to the flight.
	&  [RL2.W5.5] The RTA and EPM safety limits shall be included in the pre-brief for every test.\\\hline
\end{tabular}
\end{center}
\end{table}

\newpage
\subsection{L2W6: Level 2 Wingman Signal 6:Envelope Protection Monitor to Control Selector}
The EPM provides a signal to the CS to switch from NNCS/RTA input to Safety Pilot input when commanded by the Safety pilot (via W9) or EPM limits are violated.
\begin{table}[hbt!]
\begin{center}
\caption{\label{t:STPA_W6} W6: Envelope Protection Monitor to Control Selector}
\begin{tabular}[t]{|L{4.5cm} | L{5cm} | L{5.5cm} |}
\hline
\textbf{Unsafe Control Action}	&	\textbf{Rationale / Scenario}	&	\textbf{Requirement}	\\\hline
EPM \textbf{provides} a switch command to the CS when the pilot has not commanded it and no safety criteria are violated, resulting a a loss of test point data generation [H6].
    & This could occur when the aircraft is close to safety violations and there is noise. 
	& [RL2.W6.1] The NNCS should be trained to stay within EPM limits under noise and the RTA stay within EPM limits under noise.\\\hline
EPM \textbf{does not provide} a switch command to the CS when the pilot has commanded it or safety criteria are violated, resulting a loss of safe separation [H1], loss of control [H2], violation of geofence [H3], or harm to the pilot or aircraft [H4].
    & This could occur due to a fault in the EPM. 
	& [RL2.W6.2] The pilot shall be informed of any faults in the EPM (W8), and the EPM switch should default to output a switch to pilot control in the presence of faults.\\\hline
EPM \textbf{is too early to command} a switch command to the CS to pilot control when no safety criteria are violated, resulting a a loss of test point data generation [H6].
    & This could occur when the aircraft is close to safety violations and there is noise. 
	& [RL2.W6.3] The NNCS should be trained to stay within EPM limits under noise and the RTA stay within EPM limits under noise.\\\hline
EPM \textbf{is too late to command} a switch command to the CS when the pilot has commanded it or safety criteria are violated, resulting a loss of safe separation [H1], loss of control [H2], violation of geofence [H3], or harm to the pilot or aircraft [H4].
    & This could occur due to a fault in the EPM. 
	& [RL2.W6.4] The pilot shall be informed of any faults in the EPM (W8), and the EPM switch should default to output a switch to pilot control in the presence of faults.\\\hline
\end{tabular}
\end{center}
\end{table}

\newpage
\subsection{L2W8: Level 2 Wingman Signal 8}
\begin{table}[hbt!]
\begin{center}
\caption{\label{t:STPA_W8} W8: Envelope Protection Management to Pilot}
\begin{tabular}[t]{|L{4.5cm} | L{5cm} | L{5.5cm} |}
\hline
\textbf{Unsafe Control Action}	&	\textbf{Rationale / Scenario}	&	\textbf{Requirement}	\\\hline
EPM provides engaged/disengaged status to Pilot when the status is incorrect.	&	An error causes the EPM to provide the wrong status. If the EPM reports the status as engaged when it is not, the pilot may try to take control of the aircraft when they should not, which could jeopardize the flight test and the process of collecting test data. It may also alarm the pilot if it happens unexpectedly or if they are unable to take control, causing them to call off the flight entirely. If the EPM reports the status as disengaged when it is engaged, the pilot may not know they need to control the aircraft and it could start to lose control.	
& [RL2.W8.1] The EPM shall report the correct status to the pilot. If error caused the EPM to report the wrong status, an effort shall be made to correct the error. If it cannot be corrected, a contingency plan shall be followed	\\\hline
EPM does not provide engaged/disengaged status to Pilot when the pilot needs to know the status.	
&	An error causes the EPM to not provide the status or an error causes the status to not be displayed, even if. If the pilot does not know the status when the EPM is engaged, the pilot may not know they need to control the aircraft and the aircraft could start to lose control. If the pilot does not know the status when the EPM in disengaged, they may not be sure if the aircraft is being controlled and they may feel unsafe, which might cause them to call off the flight.	
& [RL2.W8.2] The EPM shall report its status to the pilot. If error causes it to not provide its status, an effort shall be made to correct the error. If the error cannot be corrected, a contingency plan shall be followed.	\\\hline
\end{tabular}
\end{center}
\end{table}
\subsection{L2W14: Level 2 Wingman Signal 14}
 The CS shall alert the pilot (via W14) when no signal is received (from W2).
 
\newpage
 \subsection{L1.5: Level 1 Signal 5: Lead to Wingman}
The EPM provides a signal to the CS to switch from NNCS/RTA input to Safety Pilot input when commanded by the Safety pilot (via W9) or EPM limits are violated.
\begin{table}[hbt!]
\begin{center}
\caption{\label{t:STPA_:L151} Level 1 Signal 5: Lead to Wingman (1)}
\begin{tabular}[t]{|L{3.5cm} | L{6cm} | L{5.5cm} |}
\hline
\textbf{Unsafe Control Action}	&	\textbf{Rationale / Scenario}	&	\textbf{Requirement}	\\\hline
Lead provides its position report to Wingman when it is inaccurate.	&	Data in position report could be corrupt or incorrect due to sensor error. If the wingman doesn't have an accurate position for the lead, it may fail to maintain safe separation [CCS1, CCS2], or it may try to get to a rejoin position that corresponds with the inaccurate report [H6/SC6], or it may fly through the jet wash [CCS5] and lose control.	
& [RL1.5.1]	There shall be a reasonableness check on the wingman and/or on the lead that the position report from the lead is feasible. If the wingman receives an invalid report, it shall say why and shall notify the proper controller (lead or ground station) and proceed with the proper contingency plan (maintain current flight path, return to base, loiter, etc.)	\\\hline

Lead does not provide its position report to Wingman when the wingman is in close proximity to the lead.	&	The position report might be missing because of a system error or data dropout. If the wingman doesn't have the position of the lead, it may fail to maintain safe separation [CCS1, CCS2], or it may fly through the jet wash [CCS5] and lose control.	
&  [RL1.5.2]	The wingman shall alert the flight lead pilot / and operator that it does not know where the lead is and proceed with the proper contingency plan (maintain current flight path, return to base, loiter, fly to a distant point, etc.)	\\\hline

Lead provides its position report to Wingman too early or too late when not all elements (ex. position, velocity, attitude) are up to date.	&	There could be a fault in a sensor on the lead, that is providing asynchronous updates to elements of the position report (e.g updating position and velocity at different rates), where one update doesn't make it in the frame.	& [RL1.5.3]	The elements of the position report for the lead shall be sampled at the same time step.	\\\hline

Lead provides its position report to Wingman too late when the wingman is on a collision course.	&	There could be a fault in a sensor on the lead, that is providing asynchronous updates to elements of the position report (e.g updating position and velocity at different rates), where one update doesn't make it in the frame.	& [RL1.5.4]	The wingman's operation shall have reasonable tolerance for small delays in position updates from the lead.	\\\hline

Lead (test pilot on wingman aircraft during test) provides a commanded rejoin point to Wingman when it is incorrect.	&	The data coming from the lead could be corrupted or the lead could have accidentally commanded an incorrect point.	& [RL1.5.5]	"The wingman shall not move to a rejoin point that violates safety.
The lead shall double check that the correct rejoin point is sent (e.g. as a checklist item)."	\\\hline

Lead (test pilot on wingman aircraft during test) does not provide a commanded rejoin point to Wingman when a coordinated test point has started.	&	It's possible the lead never sent the signal or that there is a data dropout.	& [RL1.5.6]	The wingman shall communicate that they do not know the rejoin point and follow the appropriate contingency plan.	\\\hline

\end{tabular}
\end{center}
\end{table}

\begin{table}[hbt!]
\begin{center}
\caption{\label{t:STPA_:L152} Level 1 Signal 5: Lead to Wingman (2)}
\begin{tabular}[t]{|L{4.5cm} | L{5cm} | L{5.5cm} |}
\hline
\textbf{Unsafe Control Action}	&	\textbf{Rationale / Scenario}	&	\textbf{Requirement}	\\\hline
Lead provides the state timestamp to Wingman when it is incorrect.	&	There could be an error in compiling the report in which the time is incorrect or isn't updated for the system. One of the aircraft may have taken off with the incorrect time.	& [RL1.5.7]	The system shall be set with the correct time before takeoff and have a method of ensuring synchronization of time during the flight.	\\\hline

Lead does not provide the state timestamp to Wingman when the wingman is in close proximity to the lead.	&	The timestamp could be left out because of a system error that leads to it not being reported or that prevents the time from being read (i.e. clock stops working). If the wingman receives a correct report without a timestamp, it won't know if that info is accurate or not, so it won't know where the lead is. Also may not be able to use the report at all, even if the rest is correct.	&[RL1.5.8]	"Instrument accuracy shall be reasonably checked prior to takeoff (e.g through regular inspection/calibration intervals). 
The lead aircraft shall check that the position report has all observations before being sent. 
If observations are missing, controllers shall be notified which are missing and why (if possible) and the lead shall attempt to send the report again. 
If errors continue to prevent attempts, steps shall be taken to correct the errors or follow an appropriate contingency plan."	\\\hline

Lead (test pilot on wingman aircraft during test) provides the test point id to Wingman when it is incorrect.	&	There was an error in the test plan or in the lead setting the test point, so the lead believes the wingman will follow one test point, while the wingman receives instructions to follow another.	&[RL1.5.9]	"Both the lead and the wingman shall have a test plan with the correct test point ids before takeoff. 
If the current id is wrong because of an error or a mistake, measures shall be taken to correct it and the report shall be sent again. If it can't be corrected, a contingency plan shall be followed."	\\\hline

Lead (test pilot on wingman aircraft during test) does not provide the test point id to Wingman when the wingman needs the test point.	&	The test point doesn't get sent because of an error or oversight. The wingman may not be able to confirm that the lead is on the same test point and may not be able to complete the test point. Or the mixup may cause delays that reduce the total number of points that can be tested in a flight.	& [RL1.5.10]	"The lead shall have the test point ids before takeoff. 
The lead aircraft shall send test points to the wingman as planned."	\\\hline

\end{tabular}
\end{center}
\end{table}

\begin{table}[hbt!]
\begin{center}
\caption{\label{t:STPA_:L153} Level 1 Signal 5: Lead to Wingman (3)}
\begin{tabular}[t]{|L{4.5cm} | L{5cm} | L{5.5cm} |}
\hline
\textbf{Unsafe Control Action}	&	\textbf{Rationale / Scenario}	&	\textbf{Requirement}	\\\hline
Lead provides its position to Wingman when it is incorrect.	&	The data could be corrupt due to transmission error, sensor error, or excess noise.	& [RL1.5.11]	"Instrument accuracy shall be reasonably checked prior to takeoff (e.g through regular inspection/calibration intervals). 
The lead aircraft shall monitor sensors for errors.
The lead aircraft shall perform a reasonableness check on the position before transmitting.
If the lead discovers a sensor error or unreasonable value for position, it shall be communicated as an invalid position in the position report.
The wingman aircraft shall perform a reasonableness check on the lead position. 
If the error is outside acceptable operational bounds, the wingman shall follow an appropriate contingency plan."	\\\hline

Lead does not provide its position to Wingman when the wingman is in close proximity to the lead.	&	The position report might be missing because of a system error or data dropout. If the wingman doesn't have the position of the lead, it may fail to maintain safe separation [CCS1, CCS2], or it may fly through the jet wash [CCS5] and lose control.	&	[RL1.5.12]	The wingman shall alert the flight lead pilot / and operator that it does not know where the lead is and proceed with the proper contingency plan.	\\\hline

Lead provides its orientation to Wingman when it is incorrect.	&	The orientation could be incorrect because of excess sensor noise, sensor error, or an error that changed the data in transmission.	& [RL1.5.13]	"Instrument accuracy shall be reasonably checked prior to takeoff (e.g through regular inspection/calibration intervals). 
The lead aircraft shall monitor sensors for errors.
The lead aircraft shall perform a reasonableness check on the orientation before transmitting.
If the lead discovers a sensor error or unreasonable value for orientation, it shall be communicated as an invalid orientation in the position report.
The wingman aircraft shall perform a reasonableness check on the lead orientation. 
If the error is outside acceptable operational bounds, the wingman shall follow an appropriate contingency plan."	\\\hline

\end{tabular}
\end{center}
\end{table}

\begin{table}[hbt!]
\begin{center}
\caption{\label{t:STPA_:L154} Level 1 Signal 5: Lead to Wingman (4)}
\begin{tabular}[t]{|L{4.5cm} | L{5cm} | L{5.5cm} |}
\hline
\textbf{Unsafe Control Action}	&	\textbf{Rationale / Scenario}	&	\textbf{Requirement}	\\\hline
Lead does not provide its orientation to Wingman when the wingman is in close proximity to the lead.	&	The orientation might not have been provided due to an error preventing the sensor from collecting data or due to an error that prevented the data from being recorded and sent.	& [RL1.5.14]	"Instrument accuracy shall be reasonably checked prior to takeoff (e.g through regular inspection/calibration intervals). 
The lead aircraft shall monitor sensors for errors.
If the wingman uncertainty for the lead aircraft orientation is outside acceptable operational bounds or cannot be estimated given a history of other data, the wingman shall follow an appropriate contingency plan."	\\\hline

Lead provides its orientation rates to Wingman when they are incorrect.	&	The orientation rate could be incorrect because of sensor error or an error that changed the data. If the wingman doesn't have the correct orientation rate, it will not be able to accurately project the path of the lead into the future, and it will be more difficult for it to maneuver safely around the lead	&  [RL1.5.15]		"Instrument accuracy shall be reasonably checked prior to takeoff (e.g through regular inspection/calibration intervals). 
The lead aircraft shall monitor sensors for errors.
The lead aircraft shall perform a reasonableness check on the orientation rates before transmitting.
If the lead discovers a sensor error or unreasonable value for orientation rates, it shall be communicated as an invalid orientation rate in the position report.
The wingman aircraft shall perform a reasonableness check on the lead orientation rates. 

If the error is outside acceptable operational bounds, the wingman shall follow an appropriate contingency plan."	\\\hline
Lead provides its true air speeds to Wingman when they are incorrect.	&	The true air speeds might be incorrect because of sensor error, calculation error, or recording error. If the wingman doesn't have the correct air speeds for the lead, it won't be able to accurately keep track of the lead's position and navigation and won't be able to safely maneuver around it.	&  [RL1.5.16]		"Instrument accuracy shall be reasonably checked prior to takeoff (e.g through regular inspection/calibration intervals). 
The lead aircraft shall monitor sensors for errors.
The lead aircraft shall perform a reasonableness check on the true air speed before transmitting.
If the lead discovers a sensor error or unreasonable value for true air speed, it shall be communicated as an invalid orientation rate in the position report.
The wingman aircraft shall perform a reasonableness check on the lead true air speed. 
If the error is outside acceptable operational bounds, the wingman shall follow an appropriate contingency plan."	\\\hline

\end{tabular}
\end{center}
\end{table}

\begin{table}[hbt!]
\begin{center}
\caption{\label{t:STPA_:L155} Level 1 Signal 5: Lead to Wingman (5)}
\begin{tabular}[t]{|L{4.5cm} | L{5cm} | L{5.5cm} |}
\hline
\textbf{Unsafe Control Action}	&	\textbf{Rationale / Scenario}	&	\textbf{Requirement}	\\\hline

Lead does not provide its true air speeds to Wingman when the wingman is in close proximity to the lead.	&	The true air speeds might be incorrect because of sensor error, calculation error, or recording error. If the wingman doesn't have the correct air speeds for the lead, it won't be able to accurately keep track of the lead's position and navigation and won't be able to safely maneuver around it.	&  [RL1.5.17]		"Instrument accuracy shall be reasonably checked prior to takeoff (e.g through regular inspection/calibration intervals). The lead aircraft shall monitor sensors for errors.
If the wingman uncertainty for the lead aircraft's true airspeed is outside acceptable operational bounds or cannot be estimated given a history of other data, the wingman shall follow an appropriate contingency plan."	\\\hline

Lead provides its velocities to Wingman when they are incorrect.	&	The velocities might be incorrect because of sensor error, calculation error, or recording error. If the wingman doesn't have the correct velocities for the lead, it won't be able to accurately keep track of the lead's position and navigation and won't be able to safely maneuver around it.	&  [RL1.5.18]		"Instrument accuracy shall be reasonably checked prior to takeoff (e.g through regular inspection/calibration intervals). 
The lead aircraft shall monitor sensors for errors.
The lead aircraft shall perform a reasonableness check on the velocities before transmitting.
If the lead discovers a sensor error or unreasonable value for velocities, it shall be communicated as an invalid orientation rate in the position report.
The wingman aircraft shall perform a reasonableness check on the lead velocities. 
If the error is outside acceptable operational bounds, the wingman shall follow an appropriate contingency plan."	\\\hline

Lead does not provide its velocities to Wingman when the wingman is in close proximity to the lead.	&	The velocities might not be provided because of sensor error, calculation error, or recording error. If the wingman doesn't have the correct velocities for the lead, it won't be able to accurately keep track of the lead's position and navigation and won't be able to safely maneuver around it.	&  [RL1.5.19]		"Instrument accuracy shall be reasonably checked prior to takeoff (e.g through regular inspection/calibration intervals). 
The lead aircraft shall monitor sensors for errors.
If the wingman uncertainty for the lead aircraft's velocities is outside acceptable operational bounds or cannot be estimated given a history of other data, the wingman shall follow an appropriate contingency plan."	\\\hline

\end{tabular}
\end{center}
\end{table}

\begin{table}[hbt!]
\begin{center}
\caption{\label{t:STPA_:L156} Level 1 Signal 5: Lead to Wingman (6)}
\begin{tabular}[t]{|L{4.5cm} | L{5cm} | L{5.5cm} |}
\hline
\textbf{Unsafe Control Action}	&	\textbf{Rationale / Scenario}	&	\textbf{Requirement}	\\\hline

Lead provides its accelerations to Wingman when it is incorrect.	&	The accelerations might be incorrect because of sensor error, calculation error, or recording error. If the wingman doesn't have the correct accelerations for the lead, it won't be able to accurately keep track of the lead's position and navigation and won't be able to safely maneuver around it.	&  [RL1.5.20]		"Instrument accuracy shall be reasonably checked prior to takeoff (e.g through regular inspection/calibration intervals). 
The lead aircraft shall monitor sensors for errors.
The lead aircraft shall perform a reasonableness check on the accelerations before transmitting.
If the lead discovers a sensor error or unreasonable value for accelerations, it shall be communicated as an invalid orientation rate in the position report.
The wingman aircraft shall perform a reasonableness check on the lead accelerations. 
If the error is outside acceptable operational bounds, the wingman shall follow an appropriate contingency plan."	\\\hline

Lead does not provide its accelerations to Wingman when the wingman is in close proximity to the lead.	&	The accelerations might not be provided because of sensor error, calculation error, or recording error. If the wingman doesn't have the correct accelerations for the lead, it won't be able to accurately keep track of the lead's position and navigation and won't be able to safely maneuver around it.	&  [RL1.5.21]		"Instrument accuracy shall be reasonably checked prior to takeoff (e.g through regular inspection/calibration intervals). 
The lead aircraft shall monitor sensors for errors.
If the wingman uncertainty for the lead aircraft's accelerations is outside acceptable operational bounds or cannot be estimated given a history of other data, the wingman shall follow an appropriate contingency plan."	\\\hline

Lead provides the amount of fuel remaining to Wingman when it is incorrect.	&	There could be an incorrect reading of the weight of the fuel due to a sensor fault or an error in compiling the report. This value being incorrect is unsafe because it provides valuable information about the state of the lead and tells the wingman whether or not the lead's behavior will change. If the actual fuel level was low, the lead might need to cut the flight short or might have performance/control issues and the fuel level will provide the wingman with some warning, in addition to other methods of communication.	&  [RL1.5.22]		"Instrument accuracy shall be reasonably checked prior to takeoff (e.g through regular inspection/calibration intervals). 
The lead aircraft shall monitor sensors for errors.
The lead aircraft shall perform a reasonableness check on the amount of fuel remaining before transmitting.
If the lead discovers a sensor error or unreasonable value for amount of fuel remaining, it shall be communicated as an invalid orientation rate in the position report.
The wingman aircraft shall perform a reasonableness check on the lead amount of fuel remaining. 
If the error is outside acceptable operational bounds, the wingman shall follow an appropriate contingency plan."	\\\hline

\end{tabular}
\end{center}
\end{table}

\begin{table}[hbt!]
\begin{center}
\caption{\label{t:STPA_:L157} Level 1 Signal 5: Lead to Wingman (7)}
\begin{tabular}[t]{|L{4.5cm} | L{5cm} | L{5.5cm} |}
\hline
\textbf{Unsafe Control Action}	&	\textbf{Rationale / Scenario}	&	\textbf{Requirement}	\\\hline

Lead does not provide the amount of fuel remaining to Wingman when the wingman is in close proximity to the lead.	&	There could be a error in the sensors or in recording that causes the amount of fuel to not be captured and sent in the report.	&  [RL1.5.23]		"Instrument accuracy shall be reasonably checked prior to takeoff (e.g through regular inspection/calibration intervals). 
The lead aircraft shall monitor sensors for errors.
If the wingman uncertainty for the lead aircraft's amount of fuel remaining is outside acceptable operational bounds or cannot be estimated given a history of other data, the wingman shall follow an appropriate contingency plan."	\\\hline

Lead provides its calibrated air speed to Wingman when it is incorrect.	&	The calibrated air speed might be incorrect because of sensor error, calculation error, or recording error. If the wingman doesn't have the correct air speed for the lead, it won't be able to accurately keep track of the lead's position and navigation and won't be able to safely maneuver around it.	&[RL1.5.24]	"Instrument accuracy shall be reasonably checked prior to takeoff (e.g through regular inspection/calibration intervals). 
The lead aircraft shall monitor sensors for errors.
The lead aircraft shall perform a reasonableness check on the calibrated air speed before transmitting.
If the lead discovers a sensor error or unreasonable value for calibrated air speed, it shall be communicated as an invalid orientation rate in the position report.
The wingman aircraft shall perform a reasonableness check on the lead calibrated air speed. 
If the error is outside acceptable operational bounds, the wingman shall follow an appropriate contingency plan."	\\\hline

Lead does not provide its calibrated air speed to Wingman when the wingman is in close proximity with the lead.	& The calibrated air speed might not be provided because of sensor error, calculation error, or recording error. If the wingman doesn't have the correct air speed for the lead, it won't be able to accurately keep track of the lead's position and navigation and won't be able to safely maneuver around it.	&[RL1.5.25]	"Instrument accuracy shall be reasonably checked prior to takeoff (e.g through regular inspection/calibration intervals). 
The lead aircraft shall monitor sensors for errors.
If the wingman uncertainty for the lead aircraft's calibrated air speed is outside acceptable operational bounds or cannot be estimated given a history of other data, the wingman shall follow an appropriate contingency plan."	\\\hline

\end{tabular}
\end{center}
\end{table}

\begin{table}[hbt!]
\begin{center}
\caption{\label{t:STPA_:L158} Level 1 Signal 5: Lead to Wingman (8)}
\begin{tabular}[t]{|L{4.5cm} | L{5cm} | L{5.5cm} |}
\hline
\textbf{Unsafe Control Action}	&	\textbf{Rationale / Scenario}	&	\textbf{Requirement}	\\\hline
Lead provides its normal accelerations to Wingman when they are incorrect.	&	The normal accelerations might be incorrect because of sensor error, calculation error, or recording error. If the wingman doesn't have the correct accelerations for the lead, it won't be able to accurately keep track of and predict the lead's position and navigation and won't be able to safely maneuver around it.	& [RL1.5.26]	"Instrument accuracy shall be reasonably checked prior to takeoff (e.g through regular inspection/calibration intervals). 
The lead aircraft shall monitor sensors for errors.
The lead aircraft shall perform a reasonableness check on the normal accelerations before transmitting.
If the lead discovers a sensor error or unreasonable value for normal accelerations, it shall be communicated as an invalid orientation rate in the position report.
The wingman aircraft shall perform a reasonableness check on the lead normal accelerations. 
If the error is outside acceptable operational bounds, the wingman shall follow an appropriate contingency plan."	\\\hline

Lead does not provide its normal accelerations to Wingman when the wingman is in close proximity to the lead.	&	The normal accelerations might not be provided because of sensor error, calculation error, or recording error. If the wingman doesn't have the correct acceleration for the lead, it won't be able to accurately keep track of and predict the lead's position and navigation and won't be able to safely maneuver around it.	& [RL1.5.27]	"Instrument accuracy shall be reasonably checked prior to takeoff (e.g through regular inspection/calibration intervals). 
The lead aircraft shall monitor sensors for errors.
If the wingman uncertainty for the lead aircraft's normal accelerations is outside acceptable operational bounds or cannot be estimated given a history of other data, the wingman shall follow an appropriate contingency plan."	\\\hline

Lead provides its PLA to Wingman when it is incorrect.	&	An error could cause the PLA value to be recorded incorrectly.	& [RL1.5.28]	"Instrument accuracy shall be reasonably checked prior to takeoff (e.g through regular inspection/calibration intervals). 
The lead aircraft shall monitor sensors for errors.
The lead aircraft shall perform a reasonableness check on the PLA before transmitting.
If the lead discovers a sensor error or unreasonable value for PLA, it shall be communicated as an invalid orientation rate in the position report.
The wingman aircraft shall perform a reasonableness check on the lead PLA. 
If the error is outside acceptable operational bounds, the wingman shall follow an appropriate contingency plan."	\\\hline

\end{tabular}
\end{center}
\end{table}

\begin{table}[hbt!]
\begin{center}
\caption{\label{t:STPA_:L159} Level 1 Signal 5: Lead to Wingman (9)}
\begin{tabular}[t]{|L{4.5cm} | L{5cm} | L{5.5cm} |}
\hline
\textbf{Unsafe Control Action}	&	\textbf{Rationale / Scenario}	&	\textbf{Requirement}	\\\hline
Lead does not provide its PLA to Wingman when the lead sends a position report.	&	An error could cause the PLA value to not be recorded.	&[RL1.5.29]	"Instrument accuracy shall be reasonably checked prior to takeoff (e.g through regular inspection/calibration intervals). The lead aircraft shall monitor sensors for errors.
If the wingman uncertainty for the lead aircraft's PLA is outside acceptable operational bounds or cannot be estimated given a history of other data, the wingman shall follow an appropriate contingency plan."	\\\hline

Lead provides its orientation angles to Wingman when they are incorrect.	&	The orientation angles might be incorrect because of sensor error, calculation error, or recording error. If the wingman doesn't have the correct orientation angles for the lead, it won't be able to accurately keep track of the lead's position and navigation and won't be able to safely maneuver around it.	& [RL1.5.30]	"Instrument accuracy shall be reasonably checked prior to takeoff (e.g through regular inspection/calibration intervals). 
The lead aircraft shall monitor sensors for errors.
The lead aircraft shall perform a reasonableness check on the orientation angles before transmitting.
If the lead discovers a sensor error or unreasonable value for orientation angles, it shall be communicated as an invalid orientation rate in the position report.
The wingman aircraft shall perform a reasonableness check on the lead orientation angles. 
If the error is outside acceptable operational bounds, the wingman shall follow an appropriate contingency plan."	\\\hline

Lead does not provide its orientation angles to Wingman when the wingman is in close proximity to the lead.	&	The orientation angles might not be provided because of sensor error, calculation error, or recording error. If the wingman doesn't have the correct orientation angles for the lead, it won't be able to accurately keep track of the lead's position and navigation and won't be able to safely maneuver around it.	& [RL1.5.31]	"Instrument accuracy shall be reasonably checked prior to takeoff (e.g through regular inspection/calibration intervals). 
The lead aircraft shall monitor sensors for errors.
If the wingman uncertainty for the lead aircraft's orientation angles is outside acceptable operational bounds or cannot be estimated given a history of other data, the wingman shall follow an appropriate contingency plan."	\\\hline

\end{tabular}
\end{center}
\end{table}

\begin{table}[hbt!]
\begin{center}
\caption{\label{t:STPA_:L1510} Level 1 Signal 5: Lead to Wingman (10)}
\begin{tabular}[t]{|L{4.5cm} | L{5cm} | L{5.5cm} |}
\hline
\textbf{Unsafe Control Action}	&	\textbf{Rationale / Scenario}	&	\textbf{Requirement}	\\\hline

Lead provides the invalid value and details to Wingman when they are incorrect.	&	Error causes the invalid value to be incorrect. If the value is set to True when the position report is accurate, the wingman won't be able to trust the report and the flight may have to be cut short. If the value is set to False when the report is incorrect, the wingman will operate on incorrect information and won't have an accurate position for the lead	& [RL1.5.32]	"Instrument accuracy shall be reasonably checked prior to takeoff (e.g through regular inspection/calibration intervals). 
The lead aircraft shall monitor sensors for errors.
The lead aircraft shall perform a reasonableness check on the invalid value and details before transmitting.
If the lead discovers a sensor error or unreasonable value for invalid value and details, it shall be communicated as an invalid orientation rate in the position report.
The wingman aircraft shall perform a reasonableness check on the lead invalid value and details. 
If the error is outside acceptable operational bounds, the wingman shall follow an appropriate contingency plan."	\\\hline

Lead does not provide the invalid value and details to Wingman when the wingman is in close proximity to the lead.	&	Error causes the invalid value to be left off of the position report. This value is used to check the validity of the report, so the wingman will be unable to trust any of the information in the report and the flight may have to be cut short	& [RL1.5.33]	"Instrument accuracy shall be reasonably checked prior to takeoff (e.g through regular inspection/calibration intervals). 
The lead aircraft shall monitor sensors for errors.
If the wingman uncertainty for the lead aircraft's invalid value and details is outside acceptable operational bounds or cannot be estimated given a history of other data, the wingman shall follow an appropriate contingency plan."	\\\hline

Lead provides its wind velocities to Wingman when they are incorrect.	&	The wind velocities might be incorrect because of sensor error, calculation error, or recording error. If the wingman doesn't have the correct wind velocities for the lead, it won't be able to accurately keep track of the lead's position and navigation and won't be able to safely maneuver around it.	& [RL1.5.34]	"Instrument accuracy shall be reasonably checked prior to takeoff (e.g through regular inspection/calibration intervals). 
The lead aircraft shall monitor sensors for errors.
The lead aircraft shall perform a reasonableness check on the wind velocities before transmitting.
If the lead discovers a sensor error or unreasonable value for wind velocities, it shall be communicated as an invalid orientation rate in the position report.
The wingman aircraft shall perform a reasonableness check on the lead wind velocities. 
If the error is outside acceptable operational bounds, the wingman shall follow an appropriate contingency plan."	\\\hline

\end{tabular}
\end{center}
\end{table}

\begin{table}[hbt!]
\begin{center}
\caption{\label{t:STPA_:L1511} Level 1 Signal 5: Lead to Wingman (11)}
\begin{tabular}[t]{|L{4.5cm} | L{5cm} | L{5.5cm} |}
\hline
\textbf{Unsafe Control Action}	&	\textbf{Rationale / Scenario}	&	\textbf{Requirement}	\\\hline

Lead does not provide its wind velocities to Wingman when the wingman is in close proximity to the lead.	&	The wind velocities might not be provided because of sensor error, calculation error, or recording error. If the wingman doesn't have the correct wind velocities for the lead, it won't be able to accurately keep track of the lead's position and navigation and won't be able to safely maneuver around it.	& [RL1.5.35]	"Instrument accuracy shall be reasonably checked prior to takeoff (e.g through regular inspection/calibration intervals). 
The lead aircraft shall monitor sensors for errors.
If the wingman uncertainty for the lead aircraft's wind velocities is outside acceptable operational bounds or cannot be estimated given a history of other data, the wingman shall follow an appropriate contingency plan."	\\\hline

Lead provides voice coordination and safety concerns to Wingman when they are unnecessary.	&	This could be due to the lead having incorrect information or not knowing what information is and isn't necessary to share. This could be unsafe because it could be distracting to both pilots and might prevent necessary information from getting through. [CCS9, CCS12]	& [RL1.5.36]	"All flight personnel shall be briefed on communication protocol before takeoff. 
Communication systems shall be tested before takeoff to ensure they work."	\\\hline

Lead does not provide voice coordination and safety concerns to Wingman when they are necessary.	&	This could be due to the lead having incorrect information or not knowing what information is and isn't necessary to share. It also could be due to communications dropout. This is unsafe because the lead and the wingman are not coordinating	&[RL1.5.37]	"All flight personnel shall be briefed on communication protocol before takeoff. 
Communication systems shall be tested before takeoff to ensure they work and measures shall be taken to fix dropouts if possible. 
If the dropout can't be fix, a contingency plan shall be followed"	\\\hline

Lead does not provide voice coordination and safety concerns to Wingman when there is a legitimate safety concern.	&	This could be due to the lead having incorrect information, being unaware of unsafe situations, or communications dropout. It's unsafe because the wingman can't be made aware of the safety concern and coordination	& [RL1.5.38]	"All flight personnel shall be briefed on communication protocol before takeoff. 
All flight personnel shall also be trained to recognize unsafe situations and be in contact with someone else who can if they are unable to recognize unsafe situations. 
Communication systems shall be tested before takeoff to ensure they work and measures shall be taken to fix dropouts if possible. 
If the dropout can't be fix, a contingency plan shall be followed"	\\\hline

Lead provides voice coordination and safety concerns to Wingman too long when some of the information is unnecessary.	&	This could be due to the lead having incorrect information or not knowing what information is and isn't necessary to share. This could be unsafe because it could be distracting to both pilots and might prevent necessary information from getting through. [CCS9, CCS12]	& [RL1.5.39]	"All flight personnel shall be briefed on communication protocol before takeoff. 
Communication systems shall be tested before takeoff to ensure they work."	\\\hline

\end{tabular}
\end{center}
\end{table}

\begin{table}[hbt!]
\begin{center}
\caption{\label{t:STPA_:L1512} Level 1 Signal 5: Lead to Wingman (12)}
\begin{tabular}[t]{|L{4.5cm} | L{5cm} | L{5.5cm} |}
\hline
\textbf{Unsafe Control Action}	&	\textbf{Rationale / Scenario}	&	\textbf{Requirement}	\\\hline

Lead provides voice coordination and safety concerns to Wingman too short when not enough detail is provided.	&	This could be due to the lead having incorrect information or not knowing what information is and isn't necessary to share. This could be unsafe because the wingman wouldn't have enough information to understand and act on the concerns and coordination.	& [RL1.5.40]	"All flight personnel shall be briefed on communication protocol before takeoff. 
If the wingman pilot needs more detail, they shall request it from the lead if possible. 
Communication systems shall be tested before takeoff to ensure they work."	\\\hline

Lead provides voice coordination and safety concerns to Wingman too early when the information is not yet relevant.	&	This could be due to the lead having incorrect information or trying to coordinate prematurely. This could be unsafe because it could be distracting to both pilots and might prevent necessary information from getting through. [CCS9, CCS12]	& [RL1.5.41]	"All flight personnel shall be briefed on communication protocol before takeoff. 
If the lead is sharing information too early, they shall stop and notify the other parties, and then repeat the information at the appropriate time. 
If the wingman tries to act on premature information, an effort shall be made to correct the mistake."	\\\hline

Lead provides voice coordination and safety concerns to Wingman too late when the event has already passed.	&	This could be due to the lead being unaware of the event or a delay in communications.	& [RL1.5.42]	"All flight personnel shall be briefed on communication protocol before takeoff. 
If the lead fails to share information on time, the wingman shall make a best effort to maintain safe flight if necessary and a contingency plan shall be followed"	\\\hline

\end{tabular}
\end{center}
\end{table}
